# Supplementary material for: An artificial intelligence framework for end-to-end rare disease phenotyping from clinical notes using large language models
Source: arXiv:2602.20324 ancillary file (2026-02-23)
Supplement: Supplementary file 1 [file Supplementary_Information.pdf]

## Supplementary Information

**Prompt for generating synthetic clinical text:**

“Generate a clinical note for a patient who is undergoing evaluation for symptoms related to rare and undiagnosed conditions. The structure of the note should vary, including both narrative and structured elements when appropriate. Integrate the following phenotypes exactly as they are listed into the narrative, each wrapped in <span class="condition"></span> tags: {Insert Human Phenotype Ontology terms here}. Ensure that the phenotypes are mentioned in context, reflecting diagnostic uncertainty or discussions about their implications, and maintaining natural language conventions.”

**Supplementary Table S1**

**Table S1.** Few-shot prompt for identifying and extracting rare disease phenotypes

| Prompt structure | Prompt text |
|---|---|
| Task specification | ### TASK: Your task is to generate an HTML version of an INPUT TEXT, using HTML <span> tags to mark up only rare disease phenotypes of a patient. |
| Markup guide | ### MARKUP GUIDE: Use <span class="phenotype"></span> to identify the phenotype. |
| Entity definition | ### DEFINITION: A rare disease phenotype includes any observable characteristic, congenital abnormality, structural variation, functional deficit, developmental condition, subjective symptom, or measurable physiological change in a patient’s health. This covers medical conditions (e.g., physical or mental abnormalities like "autism"), physical traits (e.g., "short stature," "high palate," or "long face"), congenital abnormalities (e.g., "intrauterine growth retardation," "congenital bilateral ptosis"), structural variations (e.g., "hypoplasia of the maxilla," "abnormal skull base morphology"), functional deficits (e.g., "speech apraxia," "poor suck"), developmental conditions (e.g., "global developmental delay," "growth delay"), measurable physiological changes (e.g., "decreased response to growth hormone stimulation test"), and subjective symptoms (e.g., "pain," "fatigue"). |
| Example | ### EXAMPLE INPUT TEXT: The combination of global developmental delay, neonatal seizure, and cerebral visual impairment necessitates a thorough genetic evaluation alongside metabolic testing to rule out treatable conditions. Continued support with physical and occupational therapy is recommended to address developmental delays and muscle tone issues. Recent MRI findings have shown ventriculomegaly and cerebral hypomyelination, with some evidence of progressive brain atrophy.<br><br>### EXAMPLE OUTPUT TEXT: The combination of <span class=“phenotype”>global developmental delay</span>, |

| | |
|---|---|
| | <span class="phenotype">neonatal seizure</span>, and <span class="phenotype">cerebral visual impairment</span> necessitates a thorough genetic evaluation alongside metabolic testing to rule out treatable conditions. Continued support with physical and occupational therapy is recommended to address developmental delays and muscle tone issues. Recent MRI findings have shown <span class="phenotype">ventriculomegaly</span> and <span class="phenotype">cerebral hypomyelination</span>, with some evidence of progressive <span class="phenotype">brain atrophy</span>. |
| Input note | ### INPUT TEXT: {Clinical Note} |

**<u>Supplementary Table S2</u>**

**Table S2. End-to-end performance results of RARE-PHENIX and PhenoBERT on the external validation cohort.**

| Cutoff (k) | Model | Metric | Score |
|---|---|---|---|
| 10 | ChatGPT_4o | F1 | 0.2711531 |
| 10 | ChatGPT_4o | Ontology-based Similarity Score | 0.5202793 |
| 10 | ChatGPT_4o | Precision | 0.4717041 |
| 10 | ChatGPT_4o | Recall | 0.2095202 |
| 20 | ChatGPT_4o | F1 | 0.3842606 |
| 20 | ChatGPT_4o | Ontology-based Similarity Score | 0.5871555 |
| 20 | ChatGPT_4o | Precision | 0.4559487 |
| 20 | ChatGPT_4o | Recall | 0.3709432 |
| 30 | ChatGPT_4o | F1 | 0.4220957 |
| 30 | ChatGPT_4o | Ontology-based Similarity Score | 0.6234541 |
| 30 | ChatGPT_4o | Precision | 0.4227994 |
| 30 | ChatGPT_4o | Recall | 0.4685388 |
| 40 | ChatGPT_4o | F1 | 0.4485714 |

| Cutoff (k) | Model | Metric | Score |
|---|---|---|---|
| 40 | ChatGPT_4o | Ontology-based Similarity Score | 0.6434076 |
| 40 | ChatGPT_4o | Precision | 0.4139595 |
| 40 | ChatGPT_4o | Recall | 0.5412699 |
| 50 | ChatGPT_4o | F1 | 0.4618816 |
| 50 | ChatGPT_4o | Ontology-based Similarity Score | 0.6597114 |
| 50 | ChatGPT_4o | Precision | 0.4056236 |
| 50 | ChatGPT_4o | Recall | 0.5924797 |
| 10 | Llama2_13b | F1 | 0.2813443 |
| 10 | Llama2_13b | Ontology-based Similarity Score | 0.5324238 |
| 10 | Llama2_13b | Precision | 0.4803333 |
| 10 | Llama2_13b | Recall | 0.2184373 |
| 20 | Llama2_13b | F1 | 0.3923636 |
| 20 | Llama2_13b | Ontology-based Similarity Score | 0.5902651 |
| 20 | Llama2_13b | Precision | 0.4664471 |
| 20 | Llama2_13b | Recall | 0.3758455 |
| 30 | Llama2_13b | F1 | 0.4350145 |
| 30 | Llama2_13b | Ontology-based Similarity Score | 0.6226341 |
| 30 | Llama2_13b | Precision | 0.4416712 |
| 30 | Llama2_13b | Recall | 0.4757733 |
| 40 | Llama2_13b | F1 | 0.4582229 |
| 40 | Llama2_13b | Ontology-based Similarity Score | 0.6496869 |
| 40 | Llama2_13b | Precision | 0.4296637 |
| 40 | Llama2_13b | Recall | 0.5467674 |
| 50 | Llama2_13b | F1 | 0.4659542 |

| Cutoff (k) | Model | Metric | Score |
|---|---|---|---|
| 50 | Llama2_13b | Ontology-based Similarity Score | 0.6631915 |
| 50 | Llama2_13b | Precision | 0.4194758 |
| 50 | Llama2_13b | Recall | 0.5863331 |
| 10 | Llama2_70b | F1 | 0.2878145 |
| 10 | Llama2_70b | Ontology-based Similarity Score | 0.5642585 |
| 10 | Llama2_70b | Precision | 0.4989160 |
| 10 | Llama2_70b | Recall | 0.2212029 |
| 20 | Llama2_70b | F1 | 0.4114760 |
| 20 | Llama2_70b | Ontology-based Similarity Score | 0.6295113 |
| 20 | Llama2_70b | Precision | 0.4892120 |
| 20 | Llama2_70b | Recall | 0.3929190 |
| 30 | Llama2_70b | F1 | 0.4627672 |
| 30 | Llama2_70b | Ontology-based Similarity Score | 0.6639680 |
| 30 | Llama2_70b | Precision | 0.4691586 |
| 30 | Llama2_70b | Recall | 0.4999705 |
| 40 | Llama2_70b | F1 | 0.4899003 |
| 40 | Llama2_70b | Ontology-based Similarity Score | 0.6894888 |
| 40 | Llama2_70b | Precision | 0.4601320 |
| 40 | Llama2_70b | Recall | 0.5713981 |
| 50 | Llama2_70b | F1 | 0.4994352 |
| 50 | Llama2_70b | Ontology-based Similarity Score | 0.7012748 |
| 50 | Llama2_70b | Precision | 0.4506192 |
| 50 | Llama2_70b | Recall | 0.6124012 |
| 10 | Llama2_7b | F1 | 0.2751160 |

| Cutoff (k) | Model | Metric | Score |
|---|---|---|---|
| 10 | Llama2_7b | Ontology-based Similarity Score | 0.5305220 |
| 10 | Llama2_7b | Precision | 0.4658857 |
| 10 | Llama2_7b | Recall | 0.2157390 |
| 20 | Llama2_7b | F1 | 0.3937771 |
| 20 | Llama2_7b | Ontology-based Similarity Score | 0.5932886 |
| 20 | Llama2_7b | Precision | 0.4616042 |
| 20 | Llama2_7b | Recall | 0.3848209 |
| 30 | Llama2_7b | F1 | 0.4355395 |
| 30 | Llama2_7b | Ontology-based Similarity Score | 0.6272221 |
| 30 | Llama2_7b | Precision | 0.4374362 |
| 30 | Llama2_7b | Recall | 0.4840753 |
| 40 | Llama2_7b | F1 | 0.4544760 |
| 40 | Llama2_7b | Ontology-based Similarity Score | 0.6510277 |
| 40 | Llama2_7b | Precision | 0.4246014 |
| 40 | Llama2_7b | Recall | 0.5432422 |
| 50 | Llama2_7b | F1 | 0.4600606 |
| 50 | Llama2_7b | Ontology-based Similarity Score | 0.6654405 |
| 50 | Llama2_7b | Precision | 0.4126938 |
| 50 | Llama2_7b | Recall | 0.5790017 |
| 10 | Llama31_70b | F1 | 0.2909575 |
| 10 | Llama31_70b | Ontology-based Similarity Score | 0.5520616 |
| 10 | Llama31_70b | Precision | 0.5016529 |
| 10 | Llama31_70b | Recall | 0.2234242 |
| 20 | Llama31_70b | F1 | 0.4102408 |

| Cutoff (k) | Model | Metric | Score |
|---|---|---|---|
| 20 | Llama31_70b | Ontology-based Similarity Score | 0.6255873 |
| 20 | Llama31_70b | Precision | 0.4907148 |
| 20 | Llama31_70b | Recall | 0.3913773 |
| 30 | Llama31_70b | F1 | 0.4505946 |
| 30 | Llama31_70b | Ontology-based Similarity Score | 0.6582339 |
| 30 | Llama31_70b | Precision | 0.4621494 |
| 30 | Llama31_70b | Recall | 0.4853180 |
| 40 | Llama31_70b | F1 | 0.4776145 |
| 40 | Llama31_70b | Ontology-based Similarity Score | 0.6797904 |
| 40 | Llama31_70b | Precision | 0.4551106 |
| 40 | Llama31_70b | Recall | 0.5529771 |
| 50 | Llama31_70b | F1 | 0.4896916 |
| 50 | Llama31_70b | Ontology-based Similarity Score | 0.6914596 |
| 50 | Llama31_70b | Precision | 0.4471579 |
| 50 | Llama31_70b | Recall | 0.5960360 |
| 10 | Llama31_8b | F1 | 0.2906409 |
| 10 | Llama31_8b | Ontology-based Similarity Score | 0.5404452 |
| 10 | Llama31_8b | Precision | 0.4989496 |
| 10 | Llama31_8b | Recall | 0.2238606 |
| 20 | Llama31_8b | F1 | 0.4116232 |
| 20 | Llama31_8b | Ontology-based Similarity Score | 0.6052654 |
| 20 | Llama31_8b | Precision | 0.4894937 |
| 20 | Llama31_8b | Recall | 0.3933542 |
| 30 | Llama31_8b | F1 | 0.4494766 |

| Cutoff (k) | Model | Metric | Score |
|---|---|---|---|
| 30 | Llama31_8b | Ontology-based Similarity Score | 0.6351765 |
| 30 | Llama31_8b | Precision | 0.4589115 |
| 30 | Llama31_8b | Recall | 0.4840642 |
| 40 | Llama31_8b | F1 | 0.4693854 |
| 40 | Llama31_8b | Ontology-based Similarity Score | 0.6566221 |
| 40 | Llama31_8b | Precision | 0.4451665 |
| 40 | Llama31_8b | Recall | 0.5443354 |
| 50 | Llama31_8b | F1 | 0.4827497 |
| 50 | Llama31_8b | Ontology-based Similarity Score | 0.6680001 |
| 50 | Llama31_8b | Precision | 0.4383585 |
| 50 | Llama31_8b | Recall | 0.5913368 |
| 10 | Llama32_1b | F1 | 0.1761416 |
| 10 | Llama32_1b | Ontology-based Similarity Score | 0.4121190 |
| 10 | Llama32_1b | Precision | 0.3199248 |
| 10 | Llama32_1b | Recall | 0.1313662 |
| 20 | Llama32_1b | F1 | 0.2653074 |
| 20 | Llama32_1b | Ontology-based Similarity Score | 0.4833980 |
| 20 | Llama32_1b | Precision | 0.3229950 |
| 20 | Llama32_1b | Recall | 0.2528769 |
| 30 | Llama32_1b | F1 | 0.3106874 |
| 30 | Llama32_1b | Ontology-based Similarity Score | 0.5263589 |
| 30 | Llama32_1b | Precision | 0.3128448 |
| 30 | Llama32_1b | Recall | 0.3509830 |
| 40 | Llama32_1b | F1 | 0.3343736 |

| Cutoff (k) | Model | Metric | Score |
|---|---|---|---|
| 40 | Llama32_1b | Ontology-based Similarity Score | 0.5514187 |
| 40 | Llama32_1b | Precision | 0.3047474 |
| 40 | Llama32_1b | Recall | 0.4223054 |
| 50 | Llama32_1b | F1 | 0.3459981 |
| 50 | Llama32_1b | Ontology-based Similarity Score | 0.5710885 |
| 50 | Llama32_1b | Precision | 0.2964996 |
| 50 | Llama32_1b | Recall | 0.4721468 |
| 10 | Llama32_3b | F1 | 0.2643546 |
| 10 | Llama32_3b | Ontology-based Similarity Score | 0.5004021 |
| 10 | Llama32_3b | Precision | 0.4526434 |
| 10 | Llama32_3b | Recall | 0.2070513 |
| 20 | Llama32_3b | F1 | 0.3721229 |
| 20 | Llama32_3b | Ontology-based Similarity Score | 0.5599176 |
| 20 | Llama32_3b | Precision | 0.4424979 |
| 20 | Llama32_3b | Recall | 0.3559269 |
| 30 | Llama32_3b | F1 | 0.4148982 |
| 30 | Llama32_3b | Ontology-based Similarity Score | 0.5848059 |
| 30 | Llama32_3b | Precision | 0.4237724 |
| 30 | Llama32_3b | Recall | 0.4515779 |
| 40 | Llama32_3b | F1 | 0.4329492 |
| 40 | Llama32_3b | Ontology-based Similarity Score | 0.6001832 |
| 40 | Llama32_3b | Precision | 0.4082510 |
| 40 | Llama32_3b | Recall | 0.5118606 |
| 50 | Llama32_3b | F1 | 0.4449880 |

| Cutoff (k) | Model | Metric | Score |
|---|---|---|---|
| 50 | Llama32_3b | Ontology-based Similarity Score | 0.6101592 |
| 50 | Llama32_3b | Precision | 0.4013065 |
| 50 | Llama32_3b | Recall | 0.5568390 |
| 10 | Llama33_70b | F1 | 0.2357230 |
| 10 | Llama33_70b | Ontology-based Similarity Score | 0.4921778 |
| 10 | Llama33_70b | Precision | 0.4149718 |
| 10 | Llama33_70b | Recall | 0.1798222 |
| 20 | Llama33_70b | F1 | 0.3329295 |
| 20 | Llama33_70b | Ontology-based Similarity Score | 0.5565399 |
| 20 | Llama33_70b | Precision | 0.3989987 |
| 20 | Llama33_70b | Recall | 0.3204077 |
| 30 | Llama33_70b | F1 | 0.3791821 |
| 30 | Llama33_70b | Ontology-based Similarity Score | 0.5938215 |
| 30 | Llama33_70b | Precision | 0.3843636 |
| 30 | Llama33_70b | Recall | 0.4195674 |
| 40 | Llama33_70b | F1 | 0.4046398 |
| 40 | Llama33_70b | Ontology-based Similarity Score | 0.6220690 |
| 40 | Llama33_70b | Precision | 0.3734045 |
| 40 | Llama33_70b | Recall | 0.4959789 |
| 50 | Llama33_70b | F1 | 0.4104436 |
| 50 | Llama33_70b | Ontology-based Similarity Score | 0.6369118 |
| 50 | Llama33_70b | Precision | 0.3593312 |
| 50 | Llama33_70b | Recall | 0.5371713 |
| 10 | Llama3_70b | F1 | 0.2853194 |

| Cutoff (k) | Model | Metric | Score |
|---|---|---|---|
| 10 | Llama3_70b | Ontology-based Similarity Score | 0.5570944 |
| 10 | Llama3_70b | Precision | 0.4940706 |
| 10 | Llama3_70b | Recall | 0.2184833 |
| 20 | Llama3_70b | F1 | 0.4110552 |
| 20 | Llama3_70b | Ontology-based Similarity Score | 0.6190622 |
| 20 | Llama3_70b | Precision | 0.4908331 |
| 20 | Llama3_70b | Recall | 0.3902390 |
| 30 | Llama3_70b | F1 | 0.4582605 |
| 30 | Llama3_70b | Ontology-based Similarity Score | 0.6518341 |
| 30 | Llama3_70b | Precision | 0.4670934 |
| 30 | Llama3_70b | Recall | 0.4916961 |
| 40 | Llama3_70b | F1 | 0.4808404 |
| 40 | Llama3_70b | Ontology-based Similarity Score | 0.6789156 |
| 40 | Llama3_70b | Precision | 0.4554078 |
| 40 | Llama3_70b | Recall | 0.5551104 |
| 50 | Llama3_70b | F1 | 0.4918516 |
| 50 | Llama3_70b | Ontology-based Similarity Score | 0.6935306 |
| 50 | Llama3_70b | Precision | 0.4463299 |
| 50 | Llama3_70b | Recall | 0.6000613 |
| 10 | Llama3_8b | F1 | 0.2887655 |
| 10 | Llama3_8b | Ontology-based Similarity Score | 0.5287421 |
| 10 | Llama3_8b | Precision | 0.4970075 |
| 10 | Llama3_8b | Recall | 0.2215594 |
| 20 | Llama3_8b | F1 | 0.4159184 |

| Cutoff (k) | Model | Metric | Score |
|---|---|---|---|
| 20 | Llama3_8b | Ontology-based Similarity Score | 0.5904301 |
| 20 | Llama3_8b | Precision | 0.4937713 |
| 20 | Llama3_8b | Recall | 0.3981540 |
| 30 | Llama3_8b | F1 | 0.4542898 |
| 30 | Llama3_8b | Ontology-based Similarity Score | 0.6145555 |
| 30 | Llama3_8b | Precision | 0.4638679 |
| 30 | Llama3_8b | Recall | 0.4922131 |
| 40 | Llama3_8b | F1 | 0.4796639 |
| 40 | Llama3_8b | Ontology-based Similarity Score | 0.6311961 |
| 40 | Llama3_8b | Precision | 0.4553624 |
| 40 | Llama3_8b | Recall | 0.5604488 |
| 50 | Llama3_8b | F1 | 0.4864079 |
| 50 | Llama3_8b | Ontology-based Similarity Score | 0.6404166 |
| 50 | Llama3_8b | Precision | 0.4438353 |
| 50 | Llama3_8b | Recall | 0.5985567 |
| 10 | PhenoBERT | F1 | 0.1899381 |
| 10 | PhenoBERT | Ontology-based Similarity Score | 0.4547566 |
| 10 | PhenoBERT | Precision | 0.2831978 |
| 10 | PhenoBERT | Recall | 0.1571878 |
| 20 | PhenoBERT | F1 | 0.2427707 |
| 20 | PhenoBERT | Ontology-based Similarity Score | 0.5097727 |
| 20 | PhenoBERT | Precision | 0.2531081 |
| 20 | PhenoBERT | Recall | 0.2635888 |
| 30 | PhenoBERT | F1 | 0.2602898 |

| Cutoff (k) | Model | Metric | Score |
|---|---|---|---|
| 30 | PhenoBERT | Ontology-based Similarity Score | 0.5420821 |
| 30 | PhenoBERT | Precision | 0.2334654 |
| 30 | PhenoBERT | Recall | 0.3402476 |
| 40 | PhenoBERT | F1 | 0.2643224 |
| 40 | PhenoBERT | Ontology-based Similarity Score | 0.5651375 |
| 40 | PhenoBERT | Precision | 0.2181446 |
| 40 | PhenoBERT | Recall | 0.3943542 |
| 50 | PhenoBERT | F1 | 0.2646807 |
| 50 | PhenoBERT | Ontology-based Similarity Score | 0.5766020 |
| 50 | PhenoBERT | Precision | 0.2074681 |
| 50 | PhenoBERT | Recall | 0.4385233 |

## Supplementary Table S3

**Table S3. Validation results of candidate learning-to-rank models.** Validation was performed on a patient-level 20% hold-out split from the training cohort. The model with the highest validation MAP@30 (XGBoost) was selected for external evaluation. *MAP@30 = mean average precision at 30.*

| Model | MAP@30 on the validation set |
|---|---|
| **XGBoost** | **0.848** |
| LightGBM | 0.836 |
| CatBoost | 0.811 |
| Logistic regression | 0.787 |

## Supplementary Table S4

**Table S4. Performance gains from prioritization module in RARE-PHENIX with 95% bootstrap intervals.** To assess the isolated contribution of the phenotype prioritization module (Module 3), we compared the ranked phenotype lists produced by RARE-PHENIX with a random ordering of the same extracted phenotypes. For each patient, the extracted HPO terms were randomly permuted 200 times, and performance was evaluated at top-k cutoffs (k = 10, 20, 30, 40, 50). Metrics were computed at the patient level with 95% bootstrap intervals across 1,000 bootstrap iterations.

| Cutoff | Mean | P025 | P975 | Model | MetricType |
|---|---|---|---|---|---|
| 10 | 0.07204238 | 0.055223276 | 0.08982483 | ChatGPT_4o | F1 |
| 10 | 0.11484947 | 0.090767857 | 0.13983992 | ChatGPT_4o | Precision |
| 10 | 0.05579899 | 0.040778529 | 0.07134854 | ChatGPT_4o | Recall |
| 10 | 0.08062361 | 0.059675247 | 0.10156305 | ChatGPT_4o | Ontology-based Similarity Score |
| 20 | 0.07829399 | 0.064877619 | 0.09347884 | ChatGPT_4o | F1 |
| 20 | 0.08445747 | 0.070308403 | 0.09998855 | ChatGPT_4o | Precision |
| 20 | 0.08146556 | 0.065228374 | 0.10050796 | ChatGPT_4o | Recall |
| 20 | 0.06292550 | 0.046499252 | 0.07864259 | ChatGPT_4o | Ontology-based Similarity Score |
| 30 | 0.06605094 | 0.054398031 | 0.07796812 | ChatGPT_4o | F1 |
| 30 | 0.06078441 | 0.049796183 | 0.07210007 | ChatGPT_4o | Precision |
| 30 | 0.08077881 | 0.064085837 | 0.09763575 | ChatGPT_4o | Recall |
| 30 | 0.04867281 | 0.036762996 | 0.06034728 | ChatGPT_4o | Ontology-based Similarity Score |
| 40 | 0.05052559 | 0.039824637 | 0.06152078 | ChatGPT_4o | F1 |
| 40 | 0.04202920 | 0.033127574 | 0.05125402 | ChatGPT_4o | Precision |
| 40 | 0.07063169 | 0.054593388 | 0.08705401 | ChatGPT_4o | Recall |
| 40 | 0.03481679 | 0.024743359 | 0.04593000 | ChatGPT_4o | Ontology-based Similarity Score |
| 50 | 0.04260027 | 0.031999591 | 0.05321531 | ChatGPT_4o | F1 |
| 50 | 0.03278094 | 0.024386387 | 0.04154731 | ChatGPT_4o | Precision |
| 50 | 0.07016566 | 0.053068341 | 0.08789260 | ChatGPT_4o | Recall |
| 50 | 0.02913444 | 0.020024650 | 0.03860174 | ChatGPT_4o | Ontology-based Similarity Score |
| 10 | 0.07558281 | 0.058256434 | 0.09181141 | Llama2_70b | F1 |

| Cutoff | Mean | P025 | P975 | Model | MetricType |
|---|---|---|---|---|---|
| 10 | 0.12571457 | 0.099781762 | 0.15099191 | Llama2_70b | Precision |
| 10 | 0.05720507 | 0.042060152 | 0.07133527 | Llama2_70b | Recall |
| 10 | 0.08279353 | 0.059523627 | 0.10607755 | Llama2_70b | Ontology-based Similarity Score |
| 20 | 0.08824415 | 0.073567479 | 0.10198798 | Llama2_70b | F1 |
| 20 | 0.10140573 | 0.084829611 | 0.11751767 | Llama2_70b | Precision |
| 20 | 0.08388895 | 0.067070466 | 0.09834891 | Llama2_70b | Recall |
| 20 | 0.06027512 | 0.043742464 | 0.07603782 | Llama2_70b | Ontology-based Similarity Score |
| 30 | 0.07758603 | 0.065722021 | 0.08998984 | Llama2_70b | F1 |
| 30 | 0.07406594 | 0.061755669 | 0.08645044 | Llama2_70b | Precision |
| 30 | 0.08773810 | 0.072763266 | 0.10311482 | Llama2_70b | Recall |
| 30 | 0.04124550 | 0.028310296 | 0.05379420 | Llama2_70b | Ontology-based Similarity Score |
| 40 | 0.06360510 | 0.052333496 | 0.07557711 | Llama2_70b | F1 |
| 40 | 0.05475254 | 0.044546081 | 0.06557710 | Llama2_70b | Precision |
| 40 | 0.08310860 | 0.068153035 | 0.09933199 | Llama2_70b | Recall |
| 40 | 0.03223697 | 0.021093289 | 0.04323175 | Llama2_70b | Ontology-based Similarity Score |
| 50 | 0.04860237 | 0.038459562 | 0.05897861 | Llama2_70b | F1 |
| 50 | 0.03872855 | 0.030291762 | 0.04726930 | Llama2_70b | Precision |
| 50 | 0.07248161 | 0.057361834 | 0.08864850 | Llama2_70b | Recall |
| 50 | 0.02037602 | 0.011413959 | 0.02927073 | Llama2_70b | Ontology-based Similarity Score |
| 10 | 0.08128765 | 0.066695029 | 0.09607991 | Llama3_70b | F1 |
| 10 | 0.13690443 | 0.113604622 | 0.16050525 | Llama3_70b | Precision |

| Cutoff | Mean | P025 | P975 | Model | MetricType |
|---|---|---|---|---|---|
| 10 | 0.06102133 | 0.049435359 | 0.07266332 | Llama3_70b | Recall |
| 10 | 0.08315897 | 0.060855518 | 0.10601273 | Llama3_70b | Ontology-based Similarity Score |
| 20 | 0.08650576 | 0.071910105 | 0.10071018 | Llama3_70b | F1 |
| 20 | 0.09807416 | 0.081480777 | 0.11458430 | Llama3_70b | Precision |
| 20 | 0.08335398 | 0.067274691 | 0.09860961 | Llama3_70b | Recall |
| 20 | 0.05732651 | 0.038595612 | 0.07525107 | Llama3_70b | Ontology-based Similarity Score |
| 30 | 0.07335196 | 0.059481406 | 0.08682410 | Llama3_70b | F1 |
| 30 | 0.07063400 | 0.057051506 | 0.08387682 | Llama3_70b | Precision |
| 30 | 0.08105339 | 0.062980098 | 0.09861612 | Llama3_70b | Recall |
| 30 | 0.03733453 | 0.022639948 | 0.05231756 | Llama3_70b | Ontology-based Similarity Score |
| 40 | 0.06264860 | 0.050624316 | 0.07549262 | Llama3_70b | F1 |
| 40 | 0.05362005 | 0.043104622 | 0.06523099 | Llama3_70b | Precision |
| 40 | 0.08210822 | 0.065687644 | 0.09824126 | Llama3_70b | Recall |
| 40 | 0.03002641 | 0.019014155 | 0.04062188 | Llama3_70b | Ontology-based Similarity Score |
| 50 | 0.05063911 | 0.040127508 | 0.06246293 | Llama3_70b | F1 |
| 50 | 0.04022182 | 0.031660777 | 0.05036250 | Llama3_70b | Precision |
| 50 | 0.07556900 | 0.060140398 | 0.09228924 | Llama3_70b | Recall |
| 50 | 0.02158996 | 0.012887685 | 0.03022047 | Llama3_70b | Ontology-based Similarity Score |
| 10 | 0.07027338 | 0.055254703 | 0.08578895 | Llama31_70b | F1 |
| 10 | 0.11264344 | 0.090212917 | 0.13523042 | Llama31_70b | Precision |
| 10 | 0.05440862 | 0.041835585 | 0.06798995 | Llama31_70b | Recall |

| Cutoff | Mean | P025 | P975 | Model | MetricType |
|---|---|---|---|---|---|
| 10 | 0.06233155 | 0.041811222 | 0.08285556 | Llama31_70b | Ontology-based Similarity Score |
| 20 | 0.07008280 | 0.056509588 | 0.08300695 | Llama31_70b | F1 |
| 20 | 0.07792893 | 0.063317344 | 0.09285839 | Llama31_70b | Precision |
| 20 | 0.06848103 | 0.053937413 | 0.08339071 | Llama31_70b | Recall |
| 20 | 0.04812682 | 0.033908400 | 0.06206433 | Llama31_70b | Ontology-based Similarity Score |
| 30 | 0.05737424 | 0.045177368 | 0.07048799 | Llama31_70b | F1 |
| 30 | 0.05465310 | 0.042722569 | 0.06710191 | Llama31_70b | Precision |
| 30 | 0.06452400 | 0.048060072 | 0.08134871 | Llama31_70b | Recall |
| 30 | 0.03239391 | 0.019599685 | 0.04465253 | Llama31_70b | Ontology-based Similarity Score |
| 40 | 0.04936118 | 0.037962664 | 0.06045119 | Llama31_70b | F1 |
| 40 | 0.04179422 | 0.031973125 | 0.05202229 | Llama31_70b | Precision |
| 40 | 0.06590570 | 0.050369841 | 0.08081654 | Llama31_70b | Recall |
| 40 | 0.02456779 | 0.015387817 | 0.03402901 | Llama31_70b | Ontology-based Similarity Score |
| 50 | 0.03979380 | 0.029677256 | 0.04995337 | Llama31_70b | F1 |
| 50 | 0.03120090 | 0.023037396 | 0.03955006 | Llama31_70b | Precision |
| 50 | 0.06139635 | 0.045620844 | 0.07712360 | Llama31_70b | Recall |
| 50 | 0.01701067 | 0.009004087 | 0.02521649 | Llama31_70b | Ontology-based Similarity Score |
